# Supplementary material for: One Microservice per Developer: Is This the Trend in OSS?
Source: arXiv:2308.02843 source file (2023-08-05)
Supplement: Supplementary file 1 [file Appendix.tex]

\section*{Appendix A: }
\label{sec:Appendix}

\begin{table}
 \begin{subtable}[t]{0.45\textwidth}
    \begin{tabular}{l|r|r|r|r|r|r}
        \hline
        &F1&F2&F3&F4&F5&F6\\
        \hline
         Batchfile	&	0.0395	&	0.0487	&	0.0227	&	0.0023	&	0.0929	&	0.028		\\
C	&	\textcolor{red}{\textbf{0.9958}}	&	-0.0007	&	0.0111	&	-0.0051	&	-0.017	&	0.0008	\\
C\#	&	0.0045	&	-0.0001	&	-0.0137	&	\textcolor{red}{\textbf{0.4161}}	&	-0.0116	&	-0.0036	\\
C++	&	\textcolor{red}{\textbf{0.4743}}	&	0.064	&	0.0398	&	-0.002	&	-0.0107	&	-0.0003	\\
CMake	&	\textcolor{red}{\textbf{0.9019}}	&	-0.0139	&	0.0067	&	0.0014	&	-0.0257	&	-0.0005		\\
CSS	&	0.0036	&	0.0074	&	-0.0001	&	\textcolor{red}{\textbf{0.9842}}	&	-0.0119	&	0.0097	\\
Dockerfile	&	0.0041	&	0	&	-0.0033	&	-0.0052	&	0.0057	&	-0.0012		\\
FreeMarker	&	0.0175	&	0.0062	&	0.0066	&	0.0225	&	0.0445	&	0.0033		\\
Go	&	0.0092	&	-0.0177	&	\textcolor{red}{\textbf{0.66}}	&	0.0104	&	-0.057	&	0.0029		\\
HCL	&	0.019	&	-0.0019	&	0.0406	&	-0.0047	&	\textcolor{red}{\textbf{0.9511}}	&	-0.0057	\\
HTML	&	0.0072	&	0.0049	&	0.0062	&	0.0042	&	-0.0033	&	\textcolor{red}{\textbf{0.7186}}	\\
Handlebars	&	0.0077	&	-0.0012	&	0.0023	&	-0.0188	&	-0.0165	&	0.0003		\\
Java	&	-0.0021	&	0.0201	&	-0.0003	&	0	&	0.0156	&	\textcolor{red}{\textbf{0.9945}}		\\
JavaScript	&	0.0029	&	0.004	&	-0.012	&	\textcolor{red}{\textbf{0.7218}}	&	0.0388	&	0.0018		\\
Jupyter NB	&	-0.0041	&	\textcolor{red}{\textbf{0.938}}	&	-0.0074	&	0.0032	&	-0.0023	&	0.0088		\\
Kotlin	&	-0.0012	&	0.0092	&	0.0196	&	-0.0082	&	0.003	&	0.0099		\\
Less	&	0.0003	&	-0.003	&	0.0066	&	\textcolor{red}{\textbf{0.425}}	&	0.0025	&	-0.0019		\\
Lua	&	\textcolor{red}{\textbf{0.9638}}	&	-0.0073	&	0.0005	&	-0.006	&	-0.0172	&	-0.0002		\\
Makefile	&	0.0011	&	-0.0088	&	\textcolor{red}{\textbf{0.6836}}	&	0.0105	&	-0.0306	&	0.0005		\\
Markdown	&	0.0118	&	0.3349	&	\textcolor{red}{\textbf{0.432}}	&	0.009	&	0.0349	&	0.0063		\\
Others	&	\textcolor{red}{\textbf{0.7362}}	&	0.0774	&	0.104	&	0.0202	&	0.1509	&	0.0107		\\
PLSQL	&	0.016	&	0.0112	&	0.0268	&	0.0352	&	\textcolor{red}{\textbf{0.7543}}	&	0.0166		\\
PowerShell	&	0.0026	&	-0.0114	&	0.0036	&	0.0195	&	-0.0013	&	-0.0019		\\
Python	&	0.1111	&	0.3582	&	\textcolor{red}{\textbf{0.6403}}	&	-0.0112	&	-0.0104	&	-0.0009		\\
Ruby	&	0.005	&	0.0005	&	0.025	&	-0.0087	&	0.0175	&	-0.0012		\\
Rust	&	0.0052	&	-0.0029	&	0.0284	&	-0.0283	&	0.0098	&	0.0006		\\
SCSS	&	0.0043	&	0.3694	&	0.0106	&	0.0013	&	0	&	0.005		\\
Shell	&	0.0226	&	0.0537	&	\textcolor{red}{\textbf{0.7976}}	&	-0.0209	&	\textcolor{red}{\textbf{0.5739}}	&	0.0126		\\
Smarty	&	0.0111	&	\textcolor{red}{\textbf{0.9663}}	&	0.096	&	-0.0019	&	-0.0047	&	0.0073		\\
Thrift	&	\textcolor{red}{\textbf{0.9974}}	&	-0.0104	&	0.0003	&	-0.0013	&	-0.0219	&	0		\\
TypeScript	&	0.0153	&	-0.0044	&	0.0176	&	0.1755	&	0.1077	&	-0.0012		\\
Vue	&	0.0018	&	-0.003	&	-0.005	&	0.0406	&	0.0629	&	0.0043		\\
YAML	&	0.0162	&	\textcolor{red}{\textbf{0.9487}}	&	0.182	&	0.0034	&	0.0284	&	0.0146		\\ 
\hline
    \end{tabular}
    \end{subtable}
    \\
 \begin{subtable}[t]{0.45\textwidth}
    \begin{tabular}{l|r|r|r|r|r|r|r}
        \hline
        &F7&F8&F9&F10&F11&F12&F13\\
        \hline
         Batchfile		&	0.002	&	-0.0414	&	0.0283	&	\textcolor{red}{\textbf{0.9898}}	&	-0.013	&	0.0079	&	0.0122	\\
C		&	-0.0088	&	-0.0076	&	-0.0025	&	-0.0004	&	-0.0065	&	0.0874	&	0.0219	\\
C\#	&			0.0184	&	-0.0278	&	\textcolor{red}{\textbf{0.911}}	&	-0.018	&	0.102	&	0.0008	&	-0.0406	\\
C++	&		-0.008	&	-0.0267	&	-0.006	&	-0.0102	&	-0.0229	&	\textcolor{red}{\textbf{0.8362}}	&	-0.0133	\\
CMake	&		-0.0134	&	-0.0348	&	-0.0157	&	-0.0021	&	-0.0021	&	0.0812	&	-0.0529	\\
CSS	&		-0.0371	&	0.0673	&	0.2479	&	-0.0103	&	0.0123	&	0	&	-0.031	\\
Dockerfile	&		-0.0019	&	0.0895	&	-0.0006	&	-0.0005	&	-0.0093	&	-0.0042	&	0.0024	\\
FreeMarker	&			\textcolor{red}{\textbf{0.682}}	&	0.0202	&	-0.0186	&	-0.0054	&	0.0009	&	-0.0028	&	-0.0022	\\
Go	&			0.0092	&	-0.0051	&	0.0268	&	-0.0207	&	-0.004	&	-0.0245	&	\textcolor{red}{\textbf{0.6399}}	\\
HCL	&			-0.0746	&	0.0323	&	0.0028	&	-0.0793	&	-0.0026	&	-0.004	&	0.0307	\\
HTML	&	-0.0048	&	0.0011	&	-0.0003	&	-0.0219	&	0.0022	&	-0.0007	&	0.0012	\\
Handlebars		&	0.0322	&	0.3059	&	0.0001	&	-0.0063	&	0.0424	&	0.0097	&	0.009	\\
Java	&	0.0173	&	-0.0061	&	-0.0003	&	0.0705	&	-0.0041	&	0.0021	&	-0.0062	\\
JavaScript	&	0.2283	&	0.0998	&	0.3322	&	-0.0088	&	0.0286	&	0.0029	&	-0.0323	\\
Jupyter NB		&	-0.0062	&	-0.006	&	-0.0135	&	-0.0451	&	0.0717	&	0.1918	&	0.048	\\
Kotlin		&	-0.0136	&	0.2406	&	-0.003	&	0.2579	&	0.0132	&	-0.0007	&	-0.0314	\\
Less		&	-0.0224	&	-0.0532	&	-0.1378	&	0.0056	&	0.008	&	-0.001	&	0.0083	\\
Lua	&		0.0121	&	-0.0127	&	-0.0072	&	0.0003	&	-0.004	&	0.0362	&	-0.0126	\\
Makefile		&	0.0018	&	-0.017	&	-0.0022	&	-0.0085	&	-0.0043	&	-0.0405	&	0.1574	\\
Markdown		&	0.0233	&	0.0977	&	0.0432	&	0.0838	&	0.0673	&	0.3472	&	0.2351	\\
Others		&	0.0633	&	0.2022	&	0.0655	&	0.0563	&	0.033	&	0.0537	&	0.1238	\\
PLSQL	&			0.2944	&	0.0767	&	-0.0012	&	0.1852	&	-0.011	&	0.0033	&	0.0303	\\
PowerShell	&		-0.0032	&	0.0004	&	0.0551	&	0.0015	&	0.3712	&	0.0001	&	-0.0088	\\
Python	&		0.0104	&	-0.0078	&	-0.0004	&	-0.0328	&	-0.0208	&	0.1007	&	-0.1732	\\
Ruby		&	-0.0039	&	0.0009	&	0.022	&	-0.0037	&	-0.0049	&	0.0054	&	0.195	\\
Rust	&		-0.0139	&	0.021	&	0.3541	&	0.0158	&	0.0302	&	0.0012	&	0.0616	\\
SCSS	&			0.02	&	0.0631	&	0.0139	&	-0.0018	&	\textcolor{red}{\textbf{0.9249}}	&	-0.0045	&	0.0021	\\
Shell	&	-0.0317	&	0.0103	&	0.0919	&	0.149	&	0.0472	&	0.0003	&	0.0391	\\
Smarty		&	-0.0046	&	-0.0007	&	0.0013	&	-0.0504	&	0.0803	&	-0.0814	&	-0.075	\\
Thrift		&	-0.012	&	-0.0223	&	-0.0109	&	-0.0011	&	-0.0029	&	0.0533	&	-0.0294	\\
TypeScript	&	-0.0288	&	\textcolor{red}{\textbf{0.9809}}	&	0.0648	&	0.0502	&	0.0199	&	0.0168	&	-0.0183	\\
Vue	&		\textcolor{red}{\textbf{0.8397}}	&	-0.0007	&	0.013	&	-0.0082	&	0.0059	&	0.0024	&	-0.0098	\\
YAML	&		0.0142	&	-0.0082	&	-0.0012	&	0.1778	&	0.1058	&	-0.0368	&	0.028	\\ 
\hline
    \end{tabular}
        \end{subtable}
    \caption{EFA Loadings (RQ$_2$)}
    \label{tab:loadings2}
\end{table}
